# Supplementary material for: A Simple Numerical Method for Evaluating Heat Dissipation from Curved Wires with Periodic Applied Heating
Source: arXiv:2110.04171 ancillary file (2021-10-08)
Supplement: Supplementary file 1 [file SupportingInformation.pdf]

# Supporting Information

## A Simple Numerical Method for Evaluating Heat Dissipation from Curved Wires with Periodic Applied Heating

Gabriel R. Jaffe*,[1] Victor W. Brar,[1] Max G. Lagally,[2] and Mark A. Eriksson[1]

[1]*Department of Physics, University of Wisconsin-Madison, Madison, Wisconsin 53706, USA*
[2]*Department of Materials Science and Engineering,*
*University of Wisconsin-Madison, Madison, Wisconsin 53706, USA*

*Email: gjaffe@wisc.edu

# I. FINITE WIDTH HEATER CALCULATIONS USING 2D MESHES OF POINT HEAT SOURCES

The calculations in the main text approximate a wire of finite width by evaluating the temperature at a fixed offset from an infinitely narrow wire. This approximation is valid providing that the thermal penetration depth is larger than the wire width and significantly reduces the computational cost compared to a full 2D mesh calculation. We show here that this approximation —using an infinitely narrow wire in place of a 2D mesh of width equal to the wire— is indeed valid in the range of thermal penetration depths used. Here, we show the combined effect of bending and finite width by comparing the calculation in Fig. 2(d) of the main text, which assumed an infinitely narrow wire, to calculations using a 2D mesh of point heat sources for both the straight and bent wires that better approximate a wire of finite width. The 2D mesh of point heat sources forming the wire bent at 90° can be seen in Fig. S1(a). The temperature is averaged across the width of the wire a distance $d$ from the bend in the wire. The temperature is also averaged across the width of a perfectly straight wire with the same finite width using a similar 2D mesh of point heat sources. The fractional deviations between the bent and straight finite width wires at offsets of d= 3 and 30 $\mu$m from the bend in the wire are calculated as a function of thermal penetration depth and plotted in Fig. S1(b) as open and closed circles. The fractional deviation between a bent and straight infinitely narrow wire from Fig. 2(d) in the main text is plotted for comparison (blue and red lines). These calculations show that when accounting for finite wire width the deviations near the bend (d=3 $\mu$m) differ by 0.05 between these two treatments of the wire width. The difference between the methods goes to 0 at large penetration depths, as expected.

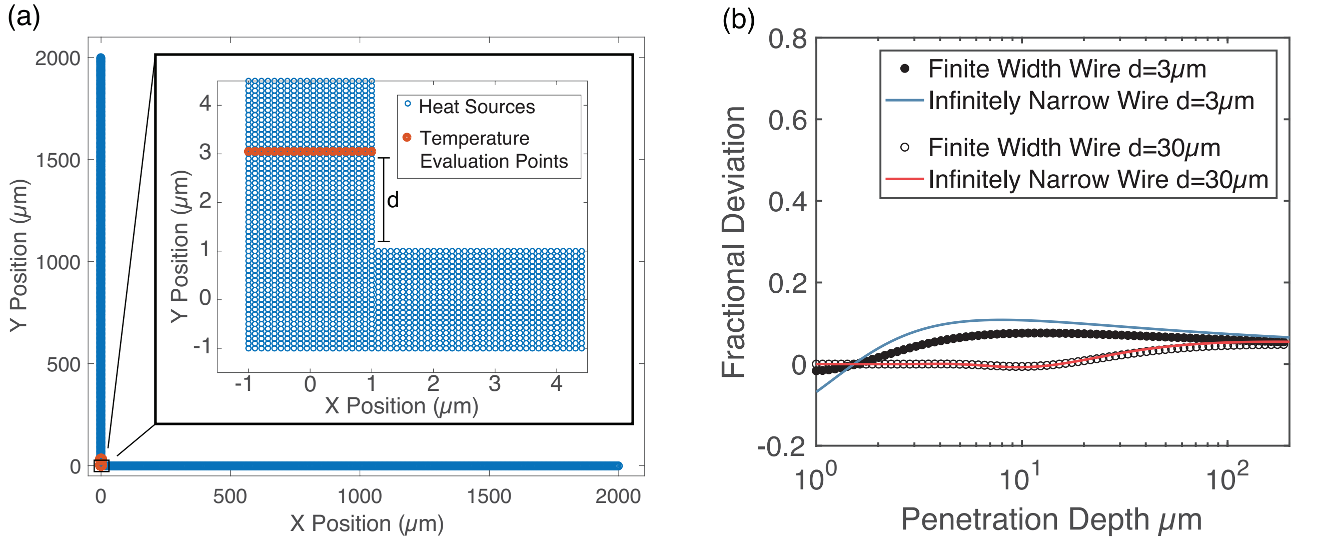


Figure S1. (a) A 2D mesh of point heat sources (blue circles) arranged to approximate a wire with a finite width of 2 $\mu$m bent at 90°. The temperature is averaged across the width of the wire at the red points a distance d=3 and d=30 $\mu$m away from the bend in the wire. The temperature is also measured at the same locations for heat sources arranged to form a perfectly straight wire with finite width 2 $\mu$m. (b) The fractional deviation (Eqn. 2 main text) between the bent finite width wire and the straight finite width wire at offsets $d$ from the bend in the wire are shown as solid and open circles, respectively. The fractional deviations at the same distances $d$ between a bent and straight infinitely narrow wire from Fig. 3(d) in the main text are shown as blue and red lines.

# II. AC POINT SOURCE HEAT-EQUATION SOLUTION

Here we derive the heat equation solution for the amplitude of the temperature oscillations about the steady state temperature for a point source of heat embedded in an infinite isotropic solid where the applied heating is periodic in time. The methodology for solving the heat equation is described in Ref. 1. We seek to solve the radially-symmetric heat equation in spherical coordinates, which can be written as

$$\frac{\partial^2 T}{\partial r^2} + \frac{2}{r}\frac{\partial T}{\partial r} = \frac{1}{D}\frac{\partial T}{\partial t}, \tag{S1}$$

where $D$ is the thermal diffusivity calculated from the thermal conductivity $\kappa$ and volumetric heat capacity $C_\rho$ as

$$D = \frac{\kappa}{C_\rho}. \tag{S2}$$

We can rewrite (S1) as

$$\frac{1}{r}\frac{\partial^2}{\partial r^2}(rT) = \frac{1}{D}\frac{\partial T}{\partial t} \tag{S3}$$

and perform the substitution

$$T = \frac{u}{r}, \tag{S4}$$

which leaves us with

$$\frac{\partial^2 u}{\partial r^2} = \frac{1}{D}\frac{\partial u}{\partial t}. \tag{S5}$$

A Laplace transform of the differential equation given in (S5) produces the subsidiary equation

$$\frac{\partial^2 \overline{u}}{\partial r^2} = \frac{p}{D}\overline{u}, \tag{S6}$$

where $p$ is the Laplace transform variable. From Ref. 1, this equation has the general solution

$$\overline{u} = e^{-Ar+B}. \tag{S7}$$

We can solve for $A$ immediately by taking the second derivative of (S7) and plugging it into (S6) yielding the condition

$$A = \sqrt{\frac{p}{D}}. \tag{S8}$$

The point source is emitting $Q$ units of heat per unit time into an infinite medium. According to Fourier's Law, the flux of heat through a spherical shell with radius r surrounding this point source is proportional to the thermal conductance of the material $G$ and the temperature differential $\partial T$ from the inside to the outside of the shell by

$$Q = -\partial T \cdot G. \tag{S9}$$

The conductance $G$ can be written in terms of the thermal conductivity $\kappa$ as

$$G = \frac{\kappa[Area]}{[thickness]} = \frac{\kappa\, 4\pi r^2}{\partial r}. \tag{S10}$$

Plugging (S10) into (S9) and rearranging we get

$$r^2\frac{\partial T}{\partial r} = -\frac{Q}{4\pi\kappa}. \tag{S11}$$

We now perform the substitution

$$T = \frac{u}{r}, \tag{S12}$$

which has derivative

$$\partial T = \frac{r\partial u - u\partial r}{r^2}. \tag{S13}$$

Plugging (S13) into (S11) we get

$$r\frac{\partial u}{\partial r} - u = -\frac{Q}{4\pi\kappa}. \tag{S14}$$

Our point source is located at the origin so, assuming $du/dr$ does not diverge, we can write

$$\lim_{r\to 0}\left(r\frac{\partial u}{\partial r}-u\right)=-\frac{Q}{4\pi\kappa} \tag{S15}$$

$$\lim_{r\to 0}u=\frac{Q}{4\pi\kappa}. \tag{S16}$$

For a sinusoidal point source that emits at a frequency $\omega$ we have

$$\lim_{r\to 0}u=\frac{Q}{4\pi\kappa}\sin(\omega t). \tag{S17}$$

The Laplace transform of (S17) is

$$\lim_{r\to 0}\overline{u}=\frac{Q}{4\pi\kappa}\frac{\omega}{p^2+\omega^2}. \tag{S18}$$

Using the general solution of $\overline{u}$ given in (S7) and setting $r$ equal to zero we solve for $B$ and find that

$$B=\ln\left(\frac{Q}{4\pi\kappa}\frac{\omega}{p^2+\omega^2}\right). \tag{S19}$$

We can now plug our expression for $A$ and $B$, given by (S8) and (S19), into the general solution of $\overline{u}$ in (S7) and get

$$\overline{u}=\frac{Q}{4\pi\kappa}\frac{\omega}{p^2+\omega^2}e^{-\sqrt{\frac{p}{D}}r}. \tag{S20}$$

We now perform the inverse Laplace transform

$$u(t)=\frac{1}{2\pi i}\frac{Q}{4\pi\kappa}\int_{\gamma-i\infty}^{\gamma+i\infty}\frac{\omega}{p^2+\omega^2}e^{-\sqrt{\frac{p}{D}}r+pt}dp. \tag{S21}$$

We solve this integral through the use of the Cauchy's residue theorem and find that

$$u(t)=\frac{Q}{4\pi\kappa}e^{-\sqrt{\frac{\omega}{2D}}r}\sin\left(\omega t-\sqrt{\frac{\omega}{2D}}r\right). \tag{S22}$$

We now reverse our substitution from (S4)

$$T=\frac{u}{r}, \tag{S23}$$

and the final solution for a point source in an infinite medium is

$$T(r,t)=\frac{Q}{4\pi\kappa}\frac{e^{-\sqrt{\frac{\omega}{2D}}r}}{r}\sin\left(\omega t-\sqrt{\frac{\omega}{2D}}r\right). \tag{S24}$$

For a semi-infinite medium, the same quantitiy of heat is flowing into half the volume of the infinite medium case, and therefore the temperatures are scaled by a factor of two:

$$\boxed{T(r,t)=\frac{Q}{2\pi\kappa}\frac{e^{-\sqrt{\frac{\omega}{2D}}r}}{r}\sin\left(\omega t-\sqrt{\frac{\omega}{2D}}r\right)}. \tag{S25}$$

Note that the surfaces of constant temperature are hemispheres that intersect the surface of the semi-infinite medium at a right angles, ensuring that the boundary condition of no heat flow out of the surface is satisfied. Eqn. (S25) here is Eqn. (1) in the main text.

## REFERENCES

[1] H. S. Carslaw and J. C. Jaeger, *Conduction of Heat in Solids* (Oxford University Press, 1947).
